# Supplementary material for: Microstructure-Resolved Degradation Simulation of Lithium-Ion Batteries in Space Applications
Source: arXiv:2111.02856 ancillary file (2022-02-04)
Supplement: Supplementary file 1 [file Supporting_Information.pdf]

# Microstructure-Resolved Degradation Simulation of Lithium-Ion Batteries in Space Applications – Supporting Information

Linda J. Bolay[a,b], Tobias Schmitt[a,b], Simon Hein[a,b], Omar S. Mendoza-Hernandez[d], Eiji Hosono[f], Daisuke Asakura[g], Koichi Kinoshita[g], Hirofumi Matsuda[g], Minoru Umeda[h], Yoshitsugu Sone[d,e], Arnulf Latz[a,b,c], Birger Horstmann[a,b,c,*]

[a]*Institute of Engineering Thermodynamics, German Aerospace Center (DLR), Pfaffenwaldring 38-40, 70569 Stuttgart, Germany*
[b]*Helmholtz Institute Ulm (HIU), Helmholtzstraße 11, 89081 Ulm, Germany*
[c]*Institute of Electrochemistry, University of Ulm, Albert-Einstein-Allee 47, 89081 Ulm, Germany*
[d]*Institute of Space and Astronautical Science, Japan Aerospace Exploration Agency, 3-1-1 Yoshinodai, Chou-ku, Sagamihara, Kanagawa 252-5210, Japan*
[e]*The Graduate University of Advanced Studies (SOKENDAI), 3-1-1 Yoshinodai, Chou-ku, Sagamihara, Kanagawa 252-5210, Japan*
[f]*Global Zero Emission Research Center, National Institute of Advanced Industrial Science and Technology (AIST), 1-1-1 Umezono, Tsukuba, Ibaraki 305-8568, Japan*
[g]*Research Institute of Energy Conservation, National Institute of Advanced Industrial Science and Technology (AIST), 1-1-1 Umezono, Tsukuba, Ibaraki 305-8568, Japan*
[h]*Department of Materials Science and Technology, Nagaoka University of Technology, 1603-1 Kamitomioka, Nagaoka, Niigata 940-2188, Japan*

## Appendix A. Model equations

In the following, we state the equations used for the P2D and the 3D model. The equations are taken from [1] and [2]. We assume constant temperature throughout the cell, which simplifies the equations in [1].

*Transport in electrolyte.*

$$\frac{\partial \varepsilon c_\mathrm{e}}{\partial t} = \nabla \cdot \left(\kappa^\mathrm{eff}\frac{t_+}{F}\nabla\varphi_\mathrm{e}\right) \;+\; \nabla \cdot \left(\left(D_\mathrm{e}^\mathrm{eff} \;-\; 2\kappa^\mathrm{eff} t_+(1-t_+)\frac{RT}{F^2}\frac{1}{c_\mathrm{e}}\right)\nabla c_\mathrm{e}\right) \qquad \text{(A.1)}$$

with the effective parameters $\kappa^\mathrm{eff} = \frac{\varepsilon}{\tau}\kappa$ and $D_\mathrm{e}^\mathrm{eff} = \frac{\varepsilon}{\tau}D_\mathrm{e}$, the ionic conductivity $\kappa$, the diffusion coefficient in electrolyte $D_\mathrm{e}$, the transference number $t_+$ (see Table B.1), the porosity $\varepsilon$ the tortuosity $\tau$, and the Li-ion concentration in electrolyte $c_\mathrm{e}$.

$$0 = \nabla \cdot \left(\kappa^\mathrm{eff}\nabla\varphi_\mathrm{e}\right) \;-\; \nabla \cdot \left(2\kappa^\mathrm{eff}(1-t_+)\frac{RT}{F}\frac{1}{c_\mathrm{e}}\nabla c_\mathrm{e}\right) \qquad \text{(A.2)}$$

with the electrochemical potential of electrolyte $\varphi_\mathrm{e}$.

*Corresponding author
*Email address:* birger.horstmann@dlr.de (Birger Horstmann)

*Transport in electrodes.*

$$\frac{\partial c_\mathrm{s}}{\partial t} = \nabla \cdot (D_\mathrm{s} \nabla c_\mathrm{s}) \tag{A.3}$$

with the Li-ion concentration in solid $c_\mathrm{s}$ and the diffusion constant in solid $D_\mathrm{s}$.

$$0 = \nabla \cdot (\sigma \nabla \Phi_\mathrm{s}) \tag{A.4}$$

with the electronic conductivity $\sigma$ and the electrical potential $\Phi_\mathrm{s}$.

*Interface reaction kinetics.* From [1] we get the interface conditions for ionic flux and electric current. The current density $i_\mathrm{se}$ across the interface of electrode and electrolyte is given by a Butler-Volmer equation:

$$i_\mathrm{se} = i_0 \left( \exp\left[\frac{\alpha F}{RT}\eta_\mathrm{s}\right] - \exp\left[-\frac{(1-\alpha)F}{RT}\eta_\mathrm{s}\right]\right) \tag{A.5}$$

with the overpotential

$$\eta_\mathrm{s} = \Phi_\mathrm{s} - \varphi_\mathrm{e} - U_0, \tag{A.6}$$

where $U_0$ is the open circuit potential (OCV). The reaction rate is

$$i_0 = k \cdot c_\mathrm{e}^\alpha c_\mathrm{s}^\alpha (c_\mathrm{s,max} - c_\mathrm{s})^{1-\alpha}, \tag{A.7}$$

with the Butler-Volmer rate constant $k$, the maximum Li concentration $c_\mathrm{s,max}$, and the charge transfer coefficient $\alpha \in [0, 1]$. Here, we assume $\alpha = 0.5$.

*OCV curves.* The OCV curves are fitted to the half cell measurements of Brown et al. [3]. They are SOC dependent with $\mathrm{SOC} = c_\mathrm{s}/c_\mathrm{s,max}$. For the anode we get

$$\begin{aligned} U_{0,\mathrm{anode}} = \; & 254.5443 - 0.02525 \cdot \mathrm{SOC} \\ & - 254.273365 \cdot \tanh((\mathrm{SOC} + 0.0097) \cdot 319.5) \\ & - 0.3086345 \cdot \tanh((\mathrm{SOC} - 0.0199) \cdot 47.0) \\ & - 0.025 \cdot \tanh((\mathrm{SOC} - 0.1414) \cdot 27.52) \\ & - 0.015 \cdot \tanh((\mathrm{SOC} - 0.2275) \cdot 18.36) \\ & - 0.1978 \cdot \tanh((\mathrm{SOC} - 1.0444) \cdot 14.43) \\ & - 0.0155 \cdot \tanh((\mathrm{SOC} - 0.56616) \cdot 12.625). \end{aligned} \tag{A.8}$$

For the cathode we get

$$\begin{aligned} U_{0,\mathrm{cathode}} = \; & 289.99 - 336.28 \cdot \mathrm{SOC} \\ & - 164.73 \cdot \tanh((\mathrm{SOC} + 0.5302) \cdot 6.824) \\ & - 0.0768 \cdot \tanh((\mathrm{SOC} - 0.442) \cdot 7.617) \\ & - 0.171 \cdot \tanh((\mathrm{SOC} - 0.9051) \cdot 13.16) \\ & - 0.3126 \cdot \tanh((\mathrm{SOC} - 0.9908) \cdot 96.14) \\ & + 3896.375 \cdot \tanh((\mathrm{SOC} - 0.36182) \cdot 0.08632). \end{aligned} \tag{A.9}$$

## Appendix B. Figures and Tables

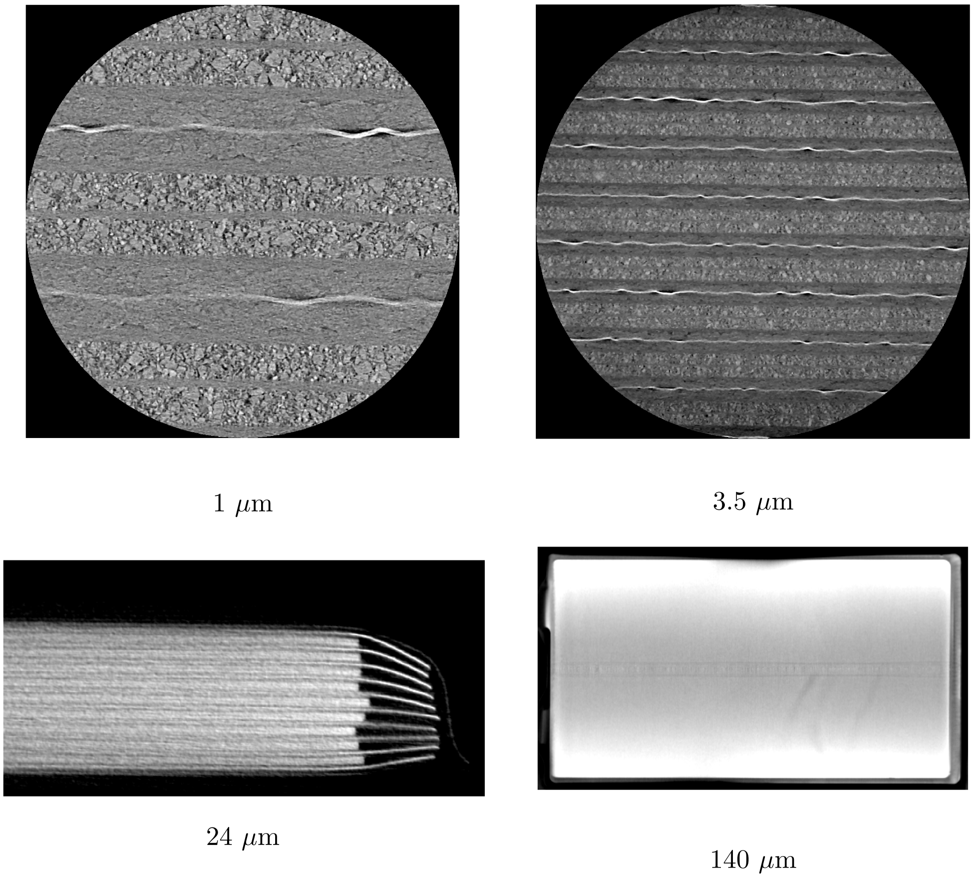


Figure B.1: CT images of satellite REIMEI's cell with different resolutions.

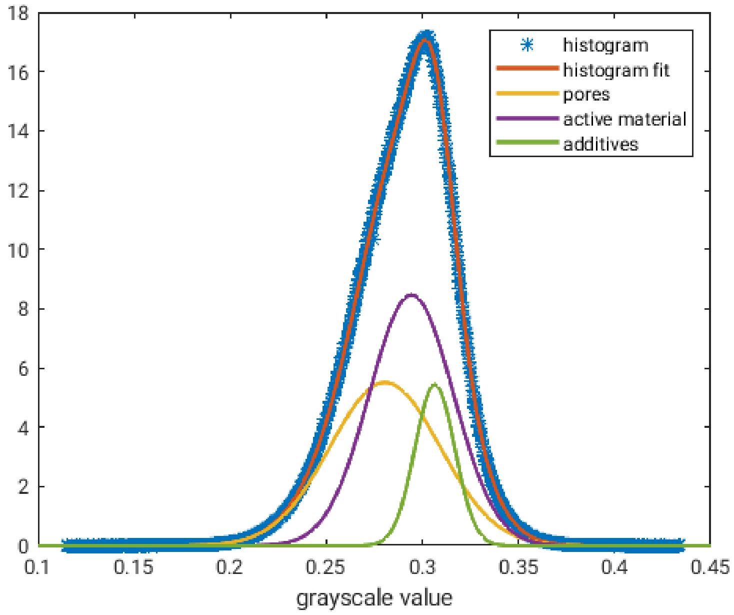


Figure B.2: Histogram of the cathode's grayvalues and the corresponding distribution approximation.

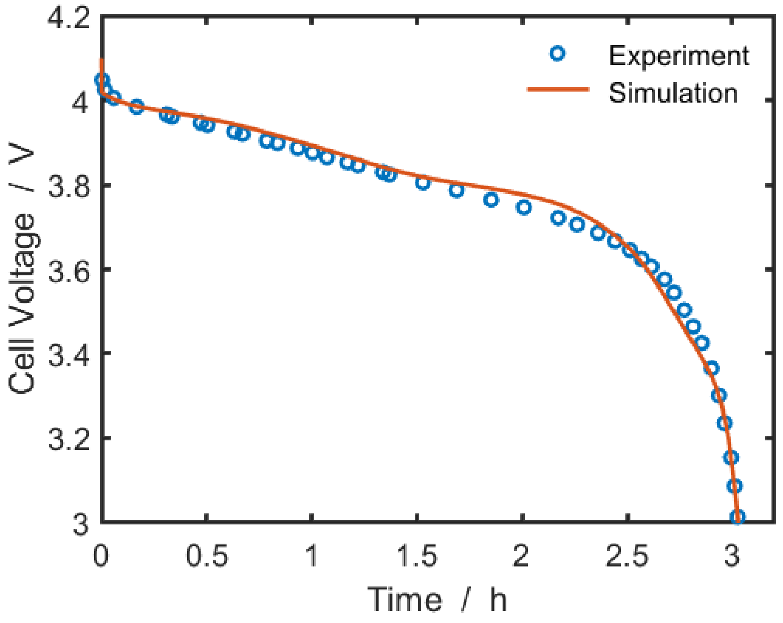


Figure B.3: Discharge curve of satellite REIMEI's cell at the beginning of cycling experiment and simulated discharge curve resulting from surrogate optimization.

| Parameter | Description | Value | Unit |
|---|---|---|---|
| $D_\mathrm{e}$ | Binary diffusion coefficient | $2.84 \cdot 10^{-10} \cdot \exp(-0.45 \cdot c_\mathrm{e})$ | $\mathrm{m^2s^{-1}}$ |
| $t_+$ | Transference number | $0.4 + 0.2 \cdot c_\mathrm{e} - 0.125 \cdot c_\mathrm{e}^2$ | 1 |
| $\kappa$ | Conductivity | $(3.4 \cdot c_\mathrm{e} - 4.7 \cdot c_\mathrm{e}^{\frac{3}{2}} + 2 \cdot c_\mathrm{e}^2) \cdot (1 + 0.2 \cdot c_\mathrm{e}^4)^{-1}$ | $\mathrm{Sm^{-1}}$ |

Table B.1: Electrolyte parameters from [2]. Parameters are concentration dependent with concentration $c_\mathrm{e}$ given in units of mol/L.

| Parameter | Description | Anode | Cathode | Sep. | Unit | Source |
|---|---|---|---|---|---|---|
| $L$ | Thickness | 45.5 | 74.5 | 30 | $10^{-6}$ m | CT data |
| $\varepsilon$ | Porosity | 0.4 | 0.4 | 0.5 | 1 | CT data |
| $\tau$ | Tortuosity | 2.6 | 2.6 | 2.6 | 1 | assumed |
| $A_\mathrm{spec}$ | Specific surface area of electrode particle | 3.03 | 2.14 | | $10^5\ \mathrm{m^2m^{-3}}$ | CT data |
| $c_\mathrm{max}$ | Maximum Li concentration | 3.161 | 2.6 | | $10^4$ mol $\mathrm{m^{-3}}$ | fit |
| $D_\mathrm{anode}$ | Diffusion coefficient of Li in electrode | 10 | 1.13 | | $10^{-13}\ \mathrm{m^2s^{-1}}$ | fit |
| $i_{00}$ | Rate constant in Butler-Volmer term | 59.2 | 4.48 | | $10^{-7} \cdot$ A $\mathrm{m^{5/2}}$ $\mathrm{mol^{-3/2}}$ | fit |
| $\mathrm{SOC}_0$ | Initial SOC | 98 | 25 | | % | fit |

Table B.2: Parameters of P2D model.

| Parameter | Description | Anode | Cathode | Unit |
|---|---|---|---|---|
| $L$ | Thickness | 50 | 58 | $10^{-6}$ m |
| $\varepsilon$ | Porosity | 0.4883 | 0.3658 | 1 |
| $A_{\text{spec}}$ | Specific surface area of electrode particle | 2.5 | 2.19 | $10^5$ $\text{m}^2\text{m}^{-3}$ |
| $c_{\max}$ | Maximum Li concentration | 3.375 | 3.16 | $10^4$ mol $\text{m}^{-3}$ |
| $D_{\text{anode}}$ | Diffusion coefficient of Li in electrode | 10 | 1.13 | $10^{-13}$ $\text{m}^2\text{s}^{-1}$ |
| $i_{00}$ | Rate constant in Butler-Volmer term | 59.2 | 4.48 | $10^{-7}\cdot$ A $\text{m}^{5/2}$ $\text{mol}^{-3/2}$ |
| $\text{SOC}_0$ | Initial SOC | 95 | 22 | % |

Table B.3: Parameters of 3D simulations.

| Parameter | Description | Value | Unit | Source |
|---|---|---|---|---|
| $V_{\text{SEI}}$ | Mean partial molar volume of the SEI | $95.86 \cdot 10^{-6}$ | $\text{m}^3\text{mol}^{-1}$ | [4] |
| $c_0^{e^-}$ | Interstitial concentration | $1.5 \cdot 10^{-2}$ | mol $\text{m}^{-3}$ | [4] |
| $s_{\text{SEI}}$ | Stoichiometric coefficient | 2 | 1 | [4] |
| $L_{\text{SEI},0}$ | Initial SEI thickness | $10 \cdot 10^{-9}$ | m | fit |
| $D^{e^-}$ | Diffusion coefficient of Li-interstitials | $1.6 \cdot 10^{-12}$ | $\text{m}^2\text{s}^{-1}$ | fit |
| $\kappa_{\text{Li}^+}^{\text{SEI}}$ | Conductivity of Li-ions in SEI | $1 \cdot 10^{-5}$ | S $\text{m}^{-1}$ | fit |

Table B.4: Parameters of degradation model.

## References


[1] A. Latz, J. Zausch, Thermodynamic consistent transport theory of Li-ion batteries, Journal of Power Sources 196 (6) (2011) 3296–3302. doi:10.1016/j.jpowsour.2010.11.088.

[2] A. Ehrl, J. Landesfeind, W. A. Wall, H. A. Gasteiger, Determination of Transport Parameters in Liquid Binary Lithium Ion Battery Electrolytes, Journal of The Electrochemical Society 164 (4) (2017) A826–A836. doi:10.1149/2.1131704jes.

[3] S. Brown, K. Ogawa, Y. Kumeuchi, S. Enomoto, M. Uno, H. Saito, Y. Sone, D. Abraham, G. Lindbergh, Cycle life evaluation of 3 Ah LixMn2O4-based lithium-ion secondary cells for low-earth-orbit satellites. II. Harvested electrode examination, Journal of Power Sources 185 (2) (2008) 1454–1464. doi:10.1016/j.jpowsour.2008.07.070.

[4] F. Single, A. Latz, B. Horstmann, Identifying the Mechanism of Continued Growth of the Solid-Electrolyte Interphase, ChemSusChem 11 (12) (2018) 1950–1955. doi:10.1002/cssc.201800077.
